# Supplementary material for: Edge-Aided Sensor Data Sharing in Vehicular Communication Networks
Source: arXiv:2206.08882 source file (2022-06-17)
Supplement: Supplementary file 1 [file 8_appendix.tex]

\begin{figure*}[ht]
\includegraphics[trim=0 0 0 0,clip,width=1\linewidth]{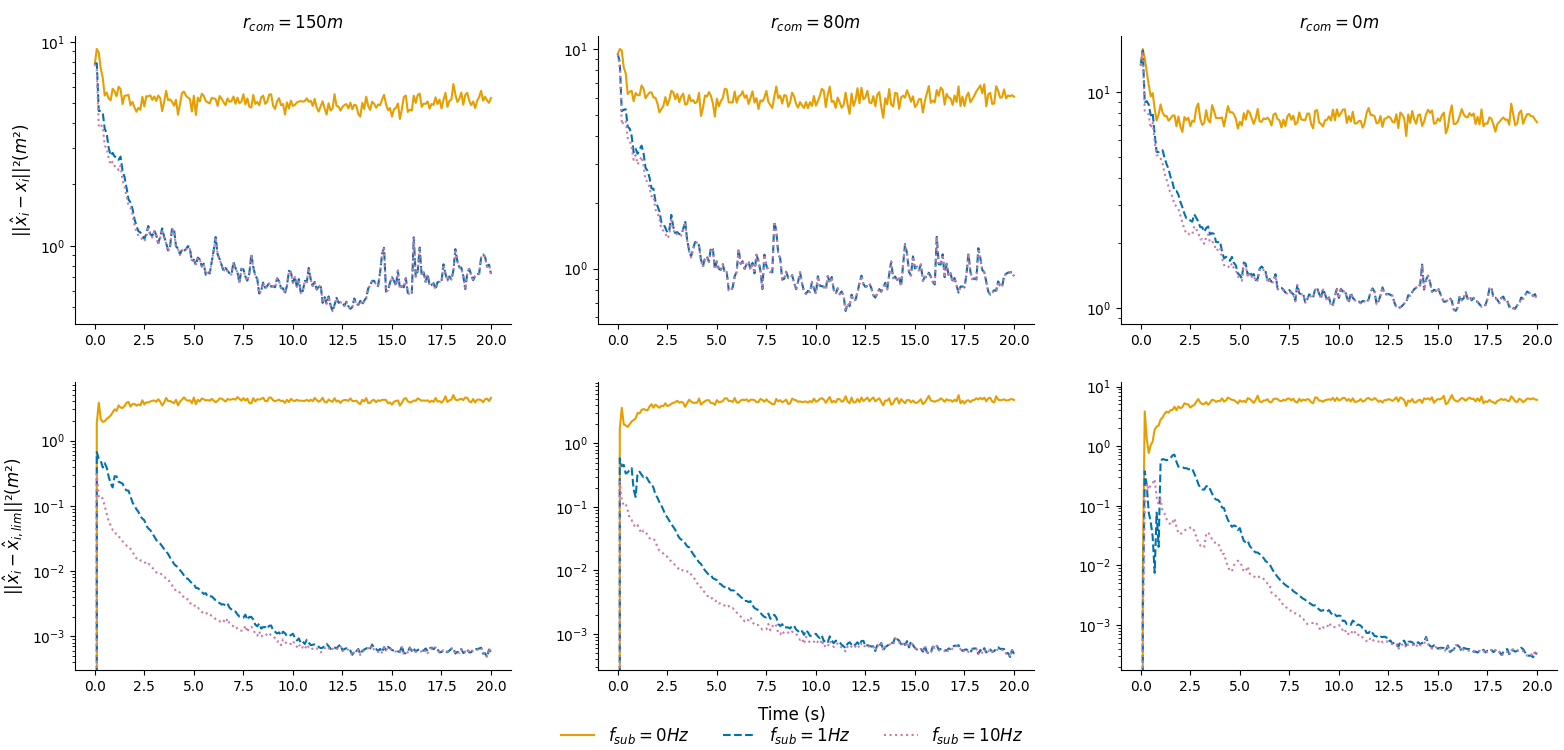}
\caption{Distributed estimation enhanced by BiFNoE. We consider the scenarios with different communication range 150\,m, 80\,m and 0\,m in three columns, where 0\,m corresponds to the case of no communication in the ad hoc network, where only local sensor data used used to estimate the targets detected. We compared the mean squared errors to the ground truth distributed estimation with subscription frequency of 10\,Hz, 1\,Hz and 0\,Hz (no subscription) in the first row and the mean squared errors to the estimation limit, where the noise ground truth is used for distributed estimation in the second row. The low-frequency subscription can still ensure that the distributed estimation converges to its limit. }
\label{fig:dist_est}
\end{figure*}

%-In Sec. IV, the authors claim that “the measurement noise values at most vehicles are relatively small and nearly constant”. And this motivates the assumption of a time-invariant covariance matrix. Could the authors provide more details (refs or data) to support this claim? Otherwise, I would consider the time-invariant covariance matrix as a technical assumption, and it would be better to state the assumption formally.
% Why does the author not consider time latency in this paper, which is significant in vehicular communication network.
%In the experiment, the article analyzes the impact of the proposed method on the network, but does not analyze the performance requirements of the edge server. Some corresponding stress tests might be helpful.
